# Supplementary material for: In-The-Field Monitoring of Functional Calls: Is It Feasible?
Source: arXiv:2001.07283 source file (2020-01-20)
Supplement: Supplementary file 1 [file Appendix01.tex]

\appendix %{Pippo}
\section{Preliminary study to select the setup} \label{app-01}

%\danyB{questo potrebbe essere il punto di partenza, per spiegare perchè poi abbiamo usato un solo buffer, e quale}

% new
As stated before, in \cite{NIER2017} we performed a preliminary study on how monitoring can affect the overhead, to search for the parameters to be used in the experiment presented in this paper. In particular, we used different buffers in the monitoring tool to save data during the monitoring phase, before flushing them in a file, to see if it can influence the results and consequently to chose the best buffer to be used in our experiment. 

% queste due frasi sotto, e la tabella, sono dal nier
Table~\ref{overheadForBuffer} shows the effectiveness of using different buffer sizes in terms of overhead and RAM consumption.
%how results change when using buffers of different sizes. 
We report the average number and percentage of \slowactions, the average overhead introduced by the monitor, and the average amount of additional RAM consumed by the monitor, measured across all the test cases and all the applications. 

% !TEX root =  ../NIER_Extension.tex

\begin{table}[h]
\resizebox{\textwidth}{!}{%
  \centering
\begin{tabular}{cccc}
        \toprule

%\begin{table}
%\caption{Effectiveness for different buffer sizes.} %\vspace{-0.3cm}
%\label{overheadForBuffer}
%\centering
%\scriptsize

%\begin{tabular}{|>{\centering}m{3em}|>{\centering}m{10em}|>{\centering}m{4em}|>{\centering\arraybackslash}m{7em}|}\hline

%{\bf buffer size (\textit{MB})} &  {\bf \slowactions \linebreak (\textit{num (\%)})} &  {\bf \ \linebreak overhead (\textit{\%})} &  {\bf RAM consumption \linebreak (\textit{MB})} \\ \hline
\textbf{Buffer size (MB)} & \textbf{\# Slow actions (\%)} & \textbf{Overhead (\%)} & \textbf{RAM consumption (MB)} \\ \midrule
0	&	20 		(18\%)		&	170\%	& 	192 \\ \midrule
1	& 	15	 	(13\%)		&	133\%	& 	198 \\  \midrule
25	&	16		(14\%)		&	104\%	&	243 \\  \midrule
50	&	17		(15\%)		&	97\%		&	281 \\  \midrule
75	&	21		(18\%)		&	128\%	&	321 \\  \midrule
100	&	16		(14\%)		&	108\%	&	355 \\  \midrule
200	&	16		(14\%)		&	93\%		&	485 \\ 

\bottomrule
\end{tabular}
}
\caption{Effectiveness for different buffer sizes.} %\vspace{-0.3cm}
\label{overheadForBuffer}
\end{table}

The percentage of \slowactions is quite stable, near $14\%$, regardless of the different sizes of the buffer. Thus, the specific size of the buffer is likely to have little impact on the results, as long as a buffer is used. In fact, the worst result is obtained when data is immediately written on file (buffer of size $0$). %For the specific set of applications that we considered, a buffer of size 50MB seems to represent a good compromise between the amount of memory consumed and the observed overhead. 

% questa era nascosta, l'ho rimaneggiata un po' e ho aggiunto l'ultima frase
According to these results, and limiting to the specific set of applications that we considered, if we exclude the configuration not using a buffer which is clearly the slowest configuration, all the other configurations perform similarly, with a buffer size of $50$MB probably presenting the best compromise between the overhead introduced in the system and the amount of additional memory consumed. While we expect the size of the buffer to be relatively important in general, as resulted from this experiment, we cannot be sure that the choice of a buffer of size of $50$MB can be generalized to all the systems: thus, for the next tests, we decided to perform tests on the same applications, and to use only this $50$MB buffer.

% questa era in nier ma qui mi pare si possa togliere
%Note that an average overhead of 14\% for a given configuration of the buffer does not correspond to a same overhead for every single action performed in each test case. Monitoring may have a different impact on different actions. This is confirmed by our observations. The average and maximum variance of the overhead internally to a same test case has been $373\%$ and $3.324\%$, respectively. This further stresses the fact that a non-intrusive monitoring technique should control the overhead on a per-action basis, and cannot be configured once for all for an application.

% questa sotto nel nier era nascosta, l'ho rimessa
Analyzing these data, we can conclude that there is a correlation between the used buffer size and the used RAM (that increases when increasing the buffer size) and with the overhead (that benefits of the usage of a buffer, since with buffer $0$ and $1$, that can be considered ``no buffer'', it is higher and then it reduces even with a buffer of $25$MB). A clear correlation between the buffer size and the number of actions overstepping their \textit{SRT} category seems not to exist. %A deeper analysis on the result regarding the actions (with respect to the SRT categories) should be performed, and this is done in the next section, when answering to the second research question.
